# Supplementary material for: LucidFusion: Reconstructing 3D Gaussians with Arbitrary Unposed Images
Source: arXiv:2410.15636 source file (2025-03-08)
Supplement: Supplementary file 1 [file appendix.tex]

\clearpage
\setcounter{page}{1}
\setcounter{figure}{0}
\setcounter{table}{0}
\maketitlesupplementary

\appendix

\section{Datasets}
The Objaverse dataset~\citep{deitke2023objaverse} contains approximately 800,000 shapes. Given the presence of numerous low-quality 3D models in the dataset (e.g., single planes, partial scans), we employed crowd workers to manually filter the dataset, focusing on objects rather than other assets like scans of large scenes or buildings. Additionally, we excluded objects that rendered predominantly in white, as this typically indicates missing textures. After filtering, our final dataset comprises approximately 98K 3D objects. 

 Using Blender, we generated synthetic images from the 3D meshes and extracted various useful annotations, including depth maps, camera intrinsics, poses, and images. We rendered these objects using a field of view (FOV) of $30^\circ$ and elevations of $-20^\circ$, $5^\circ$ and $20^\circ$, along with front views. Each elevation setting was rendered with 24 images, while the front view was rendered with 18 images, resulting in a total of 90 images per object. During training, $N$ views are randomly sampled from these 90 images. The rendered images have a resolution of $512\times 512$ and are generated under uniform lighting conditions.

\begin{table}[!ht]
    \centering
    \resizebox{\linewidth}{!}{%
    \begin{tabular}{@{}ccccc@{}}
    \toprule
                    & \makecell{w/o stage 1\\(SD~\cite{rombach2022high})} & \makecell{w. stage 1\\(SD~\cite{rombach2022high})} & \makecell{w. stage 1\\(DPT~\cite{ranftl2021visiontransformersdenseprediction})} & \makecell{w. stage 1 \\(SVD~\cite{blattmann2023stable})} \\ \midrule
    PSNR$\uparrow$  & 24.15           & \textbf{25.97}   & 24.15             & 23.96             \\
    SSIM$\uparrow$  & 0.916           & \textbf{0.930}   & 0.917             & 0.916             \\
    LPIPS$\downarrow$ & 0.080         & \textbf{0.070}   & 0.091             & 0.088             \\ \bottomrule
    \end{tabular}
    }
    \caption{Performance comparison for Stage 1 with different encoders, tested on GSO~\cite{downs2022google} dataset with sparse 4 view setting.}
    \label{tab:ablation-2}
\end{table}

\section{Implementation Details}
\paragraph{Stage 1.} Similar to~\citep{he2024lotus}, we empirically found that using a pre-trained Stable Diffusion model~\citep{rombach2022high} in a purely feedforward manner, bypassing the need for multiple diffusion steps achieves the best result, as shown in Tab.~\ref{tab:ablation-2}. The feature map $f$ is extracted before the final output layer and used by the decoder to generate Gaussian splats in Stage 2. The feature map $f$ has a shape of \(\{N, 320, \frac{H}{8}, \frac{W}{8} \}\), where $H$ and $W$ denote the image resolution. During training, we unfreeze the VAE decoder and UNet components, training the SD model in a feedforward manner without utilizing diffusion steps. Specifically, we set the text prompt to an empty string ("") and use $t=999$ for the scheduler. The RGB input views are set to 5.

\paragraph{Stage 2.} For Stage 2, the SD VAE decoder is adapted to generate Gaussian splats. We modify the SD VAE decoder to accept a channel size of 320 and output 11-channel Gaussian splat predictions, which are then processed by a Gaussian renderer to generate supervision views. During training, we randomly sample between 1 and 5 input views and render additional novel views to produce a total of 8 views for supervision. The SD and VAE decoder are trained simultaneously using only the rendering loss.

We conducted the training on 8 NVIDIA A100 (80G) GPUs for both Stage 1 and Stage 2. In Stage 1, we train the model on images with a resolution of $512\times 512$. The batch size for Stage 1 is set to 4 per GPU, resulting in an effective batch size of 32. We train for 40 epochs and Stage 1 training takes approximately 3 days. For Stage 2, we use a batch size of 2 per GPU, resulting in an effective batch size of 16, with training taking around 4 days for 20 epochs. The output 3D Gaussians are rendered at a resolution of $512\times 512$. We utilize the AdamW optimizer~\citep{loshchilov2017decoupled} with a learning rate of $3\times 10^{-5}$ for stage 1 and 2.

\begin{figure}[!t]
    \centering
    \includegraphics[width=\linewidth]{ICCV2025-Author-Kit-Feb/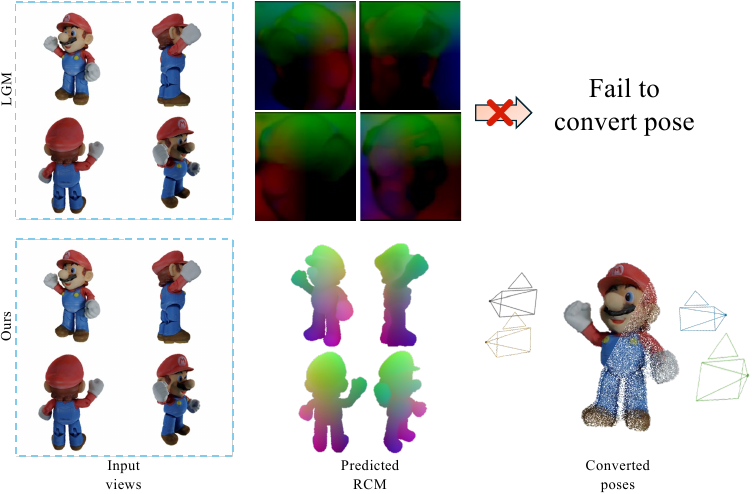}
    \captionsetup{font=small}
    \caption{Comparison with our predicted RCM and LGM centers for PnP solver, where LGM fails to resolve pose from its centers. }
    % \vspace{-0.5cm}
    \label{fig:ablation_pose_lgm}
    % \vspace{-0.2in}
\end{figure}

\section{More Visualization Results}
\paragraph{Visualization of RCM.} We visualize the predicted RCM map from input images, as shown in Fig.~\ref{fig:rcm_representation}. Starting with a set of 2D images, we predict their corresponding RCM representation within the range of $[-1, 1]$. Since the RCM representation is per-pixel aligned with the input images, we concatenate them into a shape of $[N, 6, 3]$, where $N$ is the total number of points, defined as $H \times W \times V$, with $H$, $W$, and $V$ representing the image height, width, and number of input views, respectively.

\begin{figure}[!t]
    \centering
    \includegraphics[width=\linewidth]{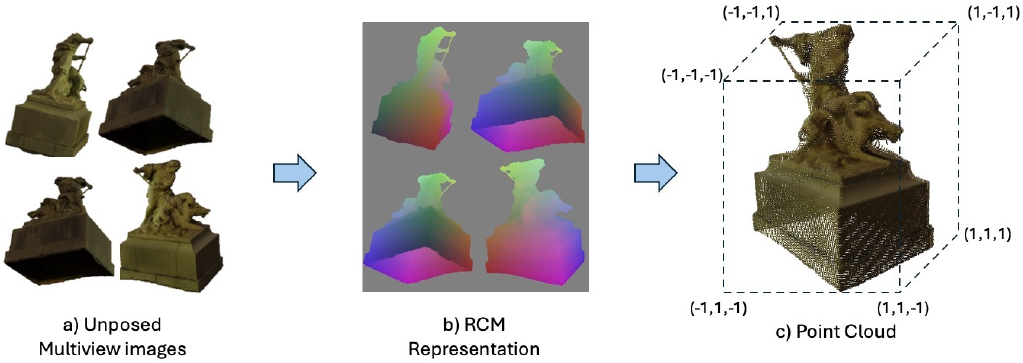}
    \captionsetup{font=small}
    \caption{Visualization of Relative Coordinate Map (RCM). }
    \label{fig:rcm_representation}
\end{figure}

\paragraph{More Cross-dataset Results.} Here we show more visualization results from various input sources in Fig.~\ref{fig:qualitative-more}.

\begin{figure*}[!t]
    \centering
    \includegraphics[width=\textwidth]{ICCV2025-Author-Kit-Feb/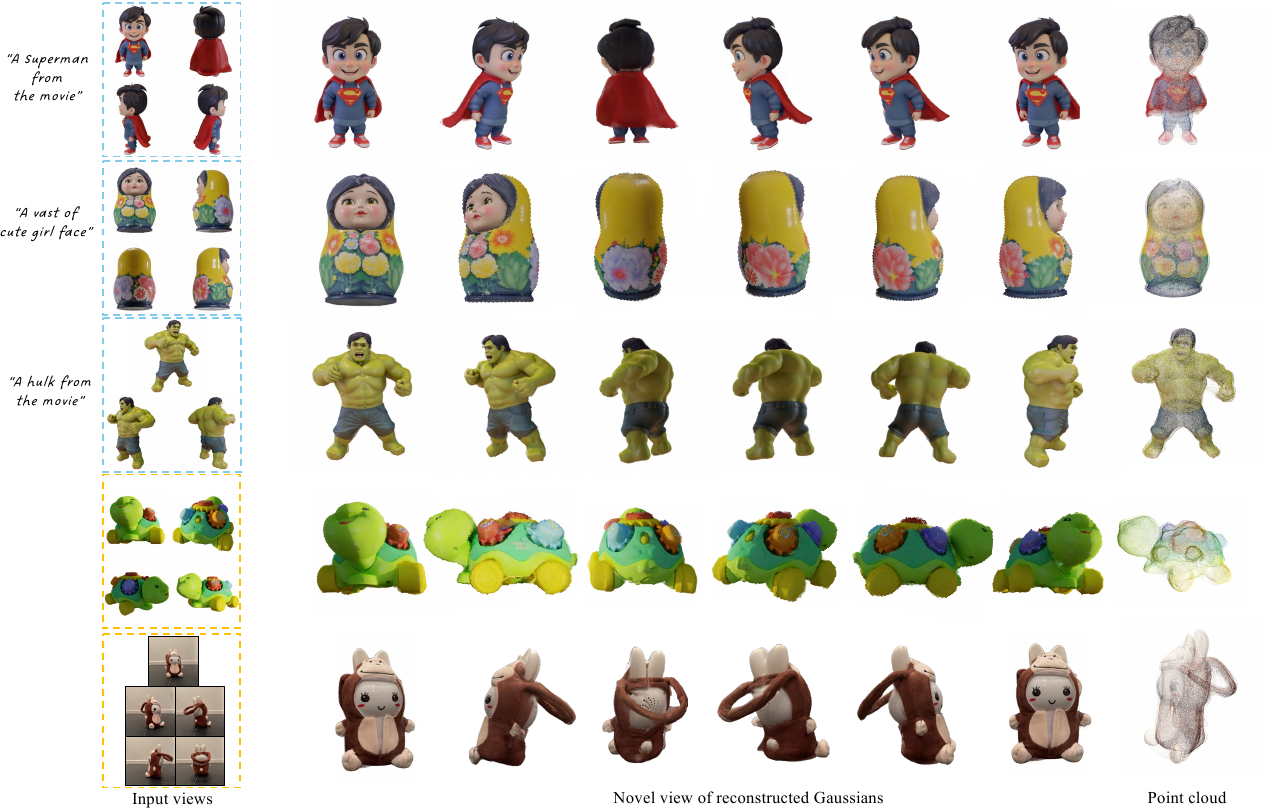}
    \captionsetup{font=small}
    \caption{More visualization results for cross-dataset generalization. Our model generalizes effectively to varying numbers of unposed input views across different data sources.}
    \label{fig:qualitative-more}
\end{figure*}

\section{Extend Abalation Study}

\paragraph{Different Encoders.} As shown in Tab.~\ref{tab:ablation-2}, we have tested different encoders, such as Stable Diffusion~\cite{rombach2022high}, Stable Video Diffusion~\cite{blattmann2023stable} and Vision Transformer (DPT)~\cite{ranftl2021visiontransformersdenseprediction}. We show that the wrapping from 2D to 3D can be learned via an image-to-image translation approach, and it can work with any genetic pre-trained vision models. We hope re-identifying this mapping can pave a new avenue for future research in the field of 3D reconstruction.

\begin{figure}[!t]
    \centering
    \includegraphics[width=\linewidth]{ICCV2025-Author-Kit-Feb/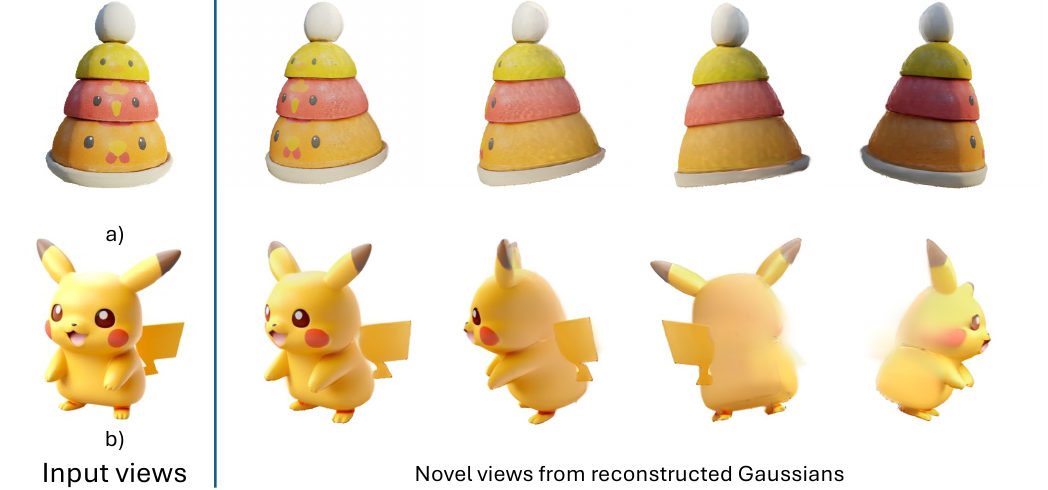}
    \captionsetup{font=small}
    \caption{Visualization of LucidFusion for single image input results without multi-view diffusion model.}
    \label{fig:ablation-single-image-pikapikapika}
\end{figure}

\paragraph{Pose Estimation from RCG.} The center extracted from RCG can be directly converted to pose via PnP solver~\cite{opencv_library}. As we show in Fig.~\ref{fig:ablation_pose_lgm}, our RCG representation remains per-pixel alignment as the input multi-views, enabling us to recover pose from it. However, in LGM~\cite{tang2024lgm}, the centers extracted from 3D Gaussians are noisy and do not remain per-pixel alignment with the input multi-views, which does not accommodate pose estimation. 

% \begin{figure*}[t]
%     % \vspace{-0.2in}
%     \centering
%     \begin{minipage}[b]{.5\textwidth}
%         \centering
%         \includegraphics[width=\linewidth]{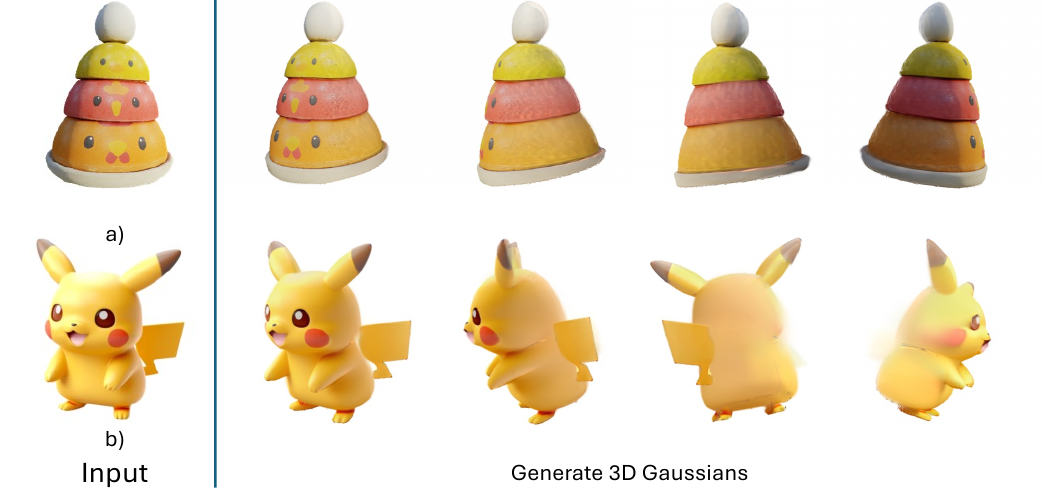}
%         \captionsetup{font=small}
%         \caption{Visualization of LucidFusion for single image input results without multi-view diffusion model.}
%         \label{fig:ablation-single-image-pikapikapika}
%     \end{minipage}
%     \hfill
%     \begin{minipage}[b]{.45\textwidth}
%         \centering
%         \includegraphics[width=\linewidth]{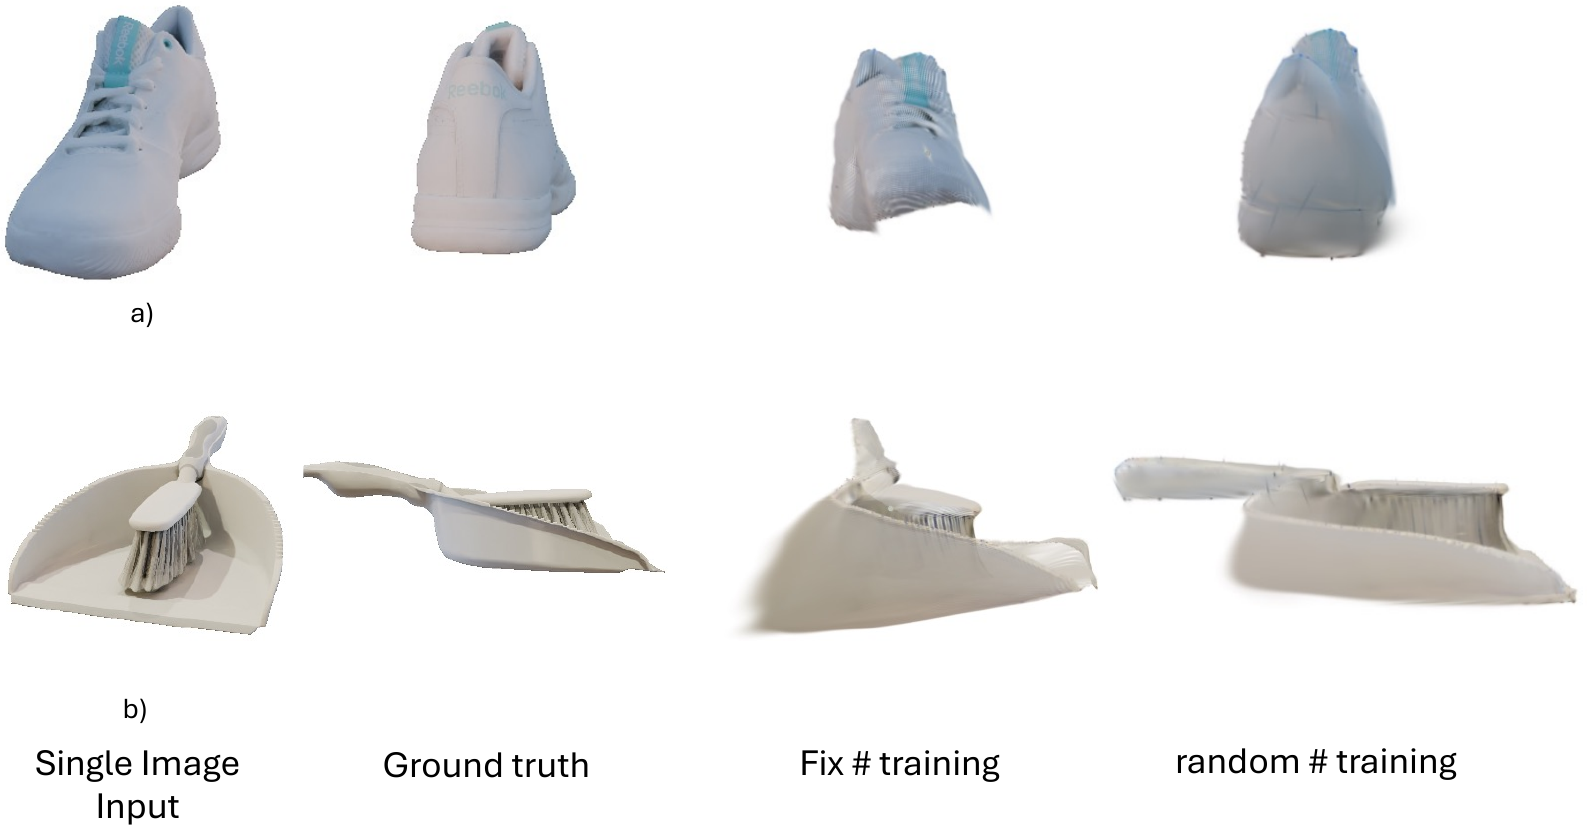}
%         \captionsetup{font=small}
%         \caption{Visualization of different training strategy results with single image input.}
%         \label{fig:single-image-abo}
%     \end{minipage}
%     % \hfill
%     % \vspace{-0.1in}
%     % \vspace{-0.2in}
% \end{figure*}

\paragraph{Number of Views.} We evaluate our model with varying numbers of input views, ranging from $i=1,2,\dots,8$ and report the performance in Tab.~\ref{tab:ablation-4}. As described in Sec.~\ref{sec:method}, our model can handle a varying number of input views, and we observe that by incorporating more views, we can further boost our reconstruction results.

\begin{table}[!t]
\centering
\small
\resizebox{\linewidth}{!}{%
\begin{tabular}{@{}ccccccc@{}}
        \toprule
        & \multicolumn{3}{c|}{Fixed Strategy} & \multicolumn{3}{c}{Random Strategy} \\
        \# of test view & PSNR$\uparrow$  & SSIM$\uparrow$  & \multicolumn{1}{c|}{LPIPS$\downarrow$} & PSNR$\uparrow$  & SSIM$\uparrow$  & LPIPS$\downarrow$ \\ \midrule
        1               & 17.36 & 0.860 & \multicolumn{1}{c|}{0.160} & 21.83 & 0.904 & 0.112 \\
        2               & 21.83 & 0.904 & \multicolumn{1}{c|}{0.080} & 23.62 & 0.915 & 0.091 \\
        4               & 25.95 & 0.932 & \multicolumn{1}{c|}{0.070} & 25.97 & 0.930 & 0.070 \\
        6               & 26.15 & 0.933 & \multicolumn{1}{c|}{0.070} & 26.11 & 0.931 & 0.070 \\ 
        8               & 26.22 & 0.933 & \multicolumn{1}{c|}{0.070} & \textbf{26.25} & \textbf{0.933} & \textbf{0.069} \\ \bottomrule
        \end{tabular}%
        }
        \captionsetup{font=small}
        \caption{Comparison between different training strategy with number of input views.}
        % \vspace{-0.5cm}
        \label{tab:ablation-4}
\end{table}

\begin{figure}[!thb]
    \centering
    \includegraphics[width=\linewidth]{ICCV2025-Author-Kit-Feb/figure/single_image_abo_crop.pdf}
    \captionsetup{font=small}
    \caption{Visualization of different training strategy results with single image input.}
    \label{fig:single-image-abo}
\end{figure}

\paragraph{Training with Random Views.} We evaluate our model's performance in Stage 2 training under fixed and random input view settings. In the fixed strategy, we train for 20 epochs with 5 input views, while in the random strategy, we randomly sample between 1 and 5 views per batch over 20 epochs. 
The results, shown in Tab.~\ref{tab:ablation-4}, indicate that the model trained with random input views performs better when the number of views is limited. Notably, with only a single input view, the model trained with random views outperforms the fixed views by a large margin. However, when the input views provide sufficient coverage of the object, both models exhibit comparable performance. 

As demonstrated in Fig.~\ref{fig:single-image-abo}, the model trained with a fixed number of views struggles to predict unseen regions, whereas the random view training strategy still produces reasonable predictions for those regions. It is important to note that single-image reconstruction is inherently ill-posed; while the model can faithfully reconstruct seen regions, it may fail in unseen areas. Nonetheless, LucidFusion provides reliable predictions under such conditions, showcasing its superior performance. Additional results for single-image input across various data sources are presented in Fig.~\ref{fig:ablation-single-image-pikapikapika}.
